# Supplementary material for: ALAS: A Stateful Multi-LLM Agent Framework for Disruption-Aware Planning
Source: arXiv:2505.12501 source file (2025-05-18)
Supplement: Supplementary file 2 [file AppendixValidationRefinement.tex]

\section{Phase Validation and Refinement}
\label{app:vlidation-spec}
